# Supplementary material for: CAT-Seg: Cost Aggregation for Open-Vocabulary Semantic Segmentation
Source: arXiv:2303.11797 source file (2024-03-31)
Supplement: Supplementary file 4 [file inference_ablation.tex]

\begin{table}[H]
    \centering
    \resizebox{\linewidth}{!}{
   \begin{tabular}{l|cccccc}
        \toprule
        Methods & A-847 & PC-459 & A-150 & PC-59 & PAS-20 & $\textnormal{PAS-20}^b$
         \\
        \midrule\midrule
        \ours w/ training reso. & \underline{14.6}& \underline{22.1}& \underline{35.7}& \underline{60.9}& \underline{96.3}& \underline{79.9}\\
        \hlrow Ours & \textbf{16.0}& \textbf{23.8}& \textbf{37.9}& \textbf{63.3}& \textbf{97.0}& \textbf{82.5}\\
        \bottomrule
\end{tabular}
}%
\vspace{-5pt}
        \caption{\textbf{Ablation study of inference strategy.} CLIP with ViT-L is used for ablation.}
    \label{tab:inference-ablation}
    \vspace{-10pt}
\end{table}
