# Supplementary material for: CAT-Seg: Cost Aggregation for Open-Vocabulary Semantic Segmentation
Source: arXiv:2303.11797 source file (2024-03-31)
Supplement: Supplementary file 7 [file patch_inference.tex]

\begin{figure}[t]
    \centering
    \includegraphics[width=1.0\linewidth]{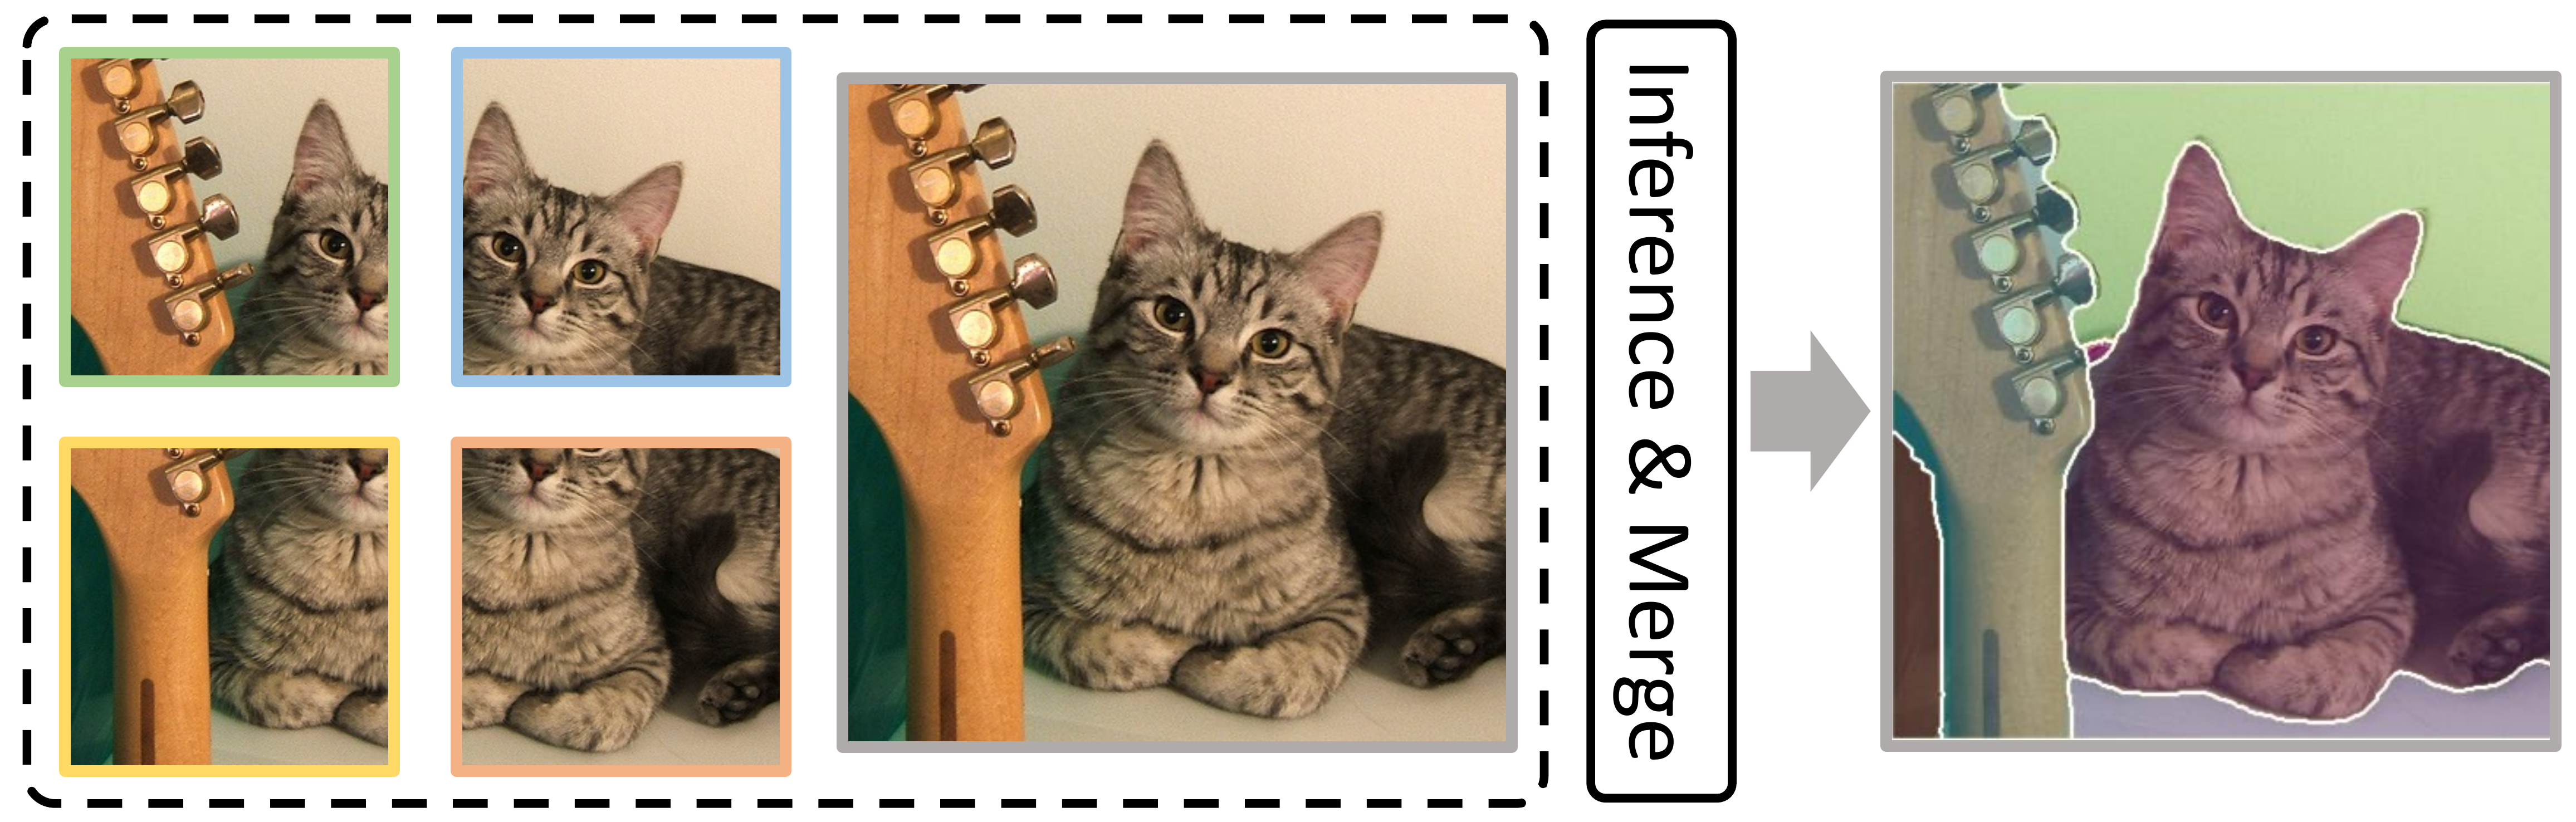}\hfill\\
    \vspace{-5pt}
    \caption{\textbf{Illustration of the patch inference.} During inference, we divide the input image into patches, thereby increasing the effective resolution.}
    \label{fig:patch-inference}
    \vspace{-10pt}
\end{figure}
