# Supplementary material for: CAT-Seg: Cost Aggregation for Open-Vocabulary Semantic Segmentation
Source: arXiv:2303.11797 source file (2024-03-31)
Supplement: Supplementary file 9 [file pc59.tex]

\begin{figure*}
    \centering
    \includegraphics[width=0.95\linewidth]{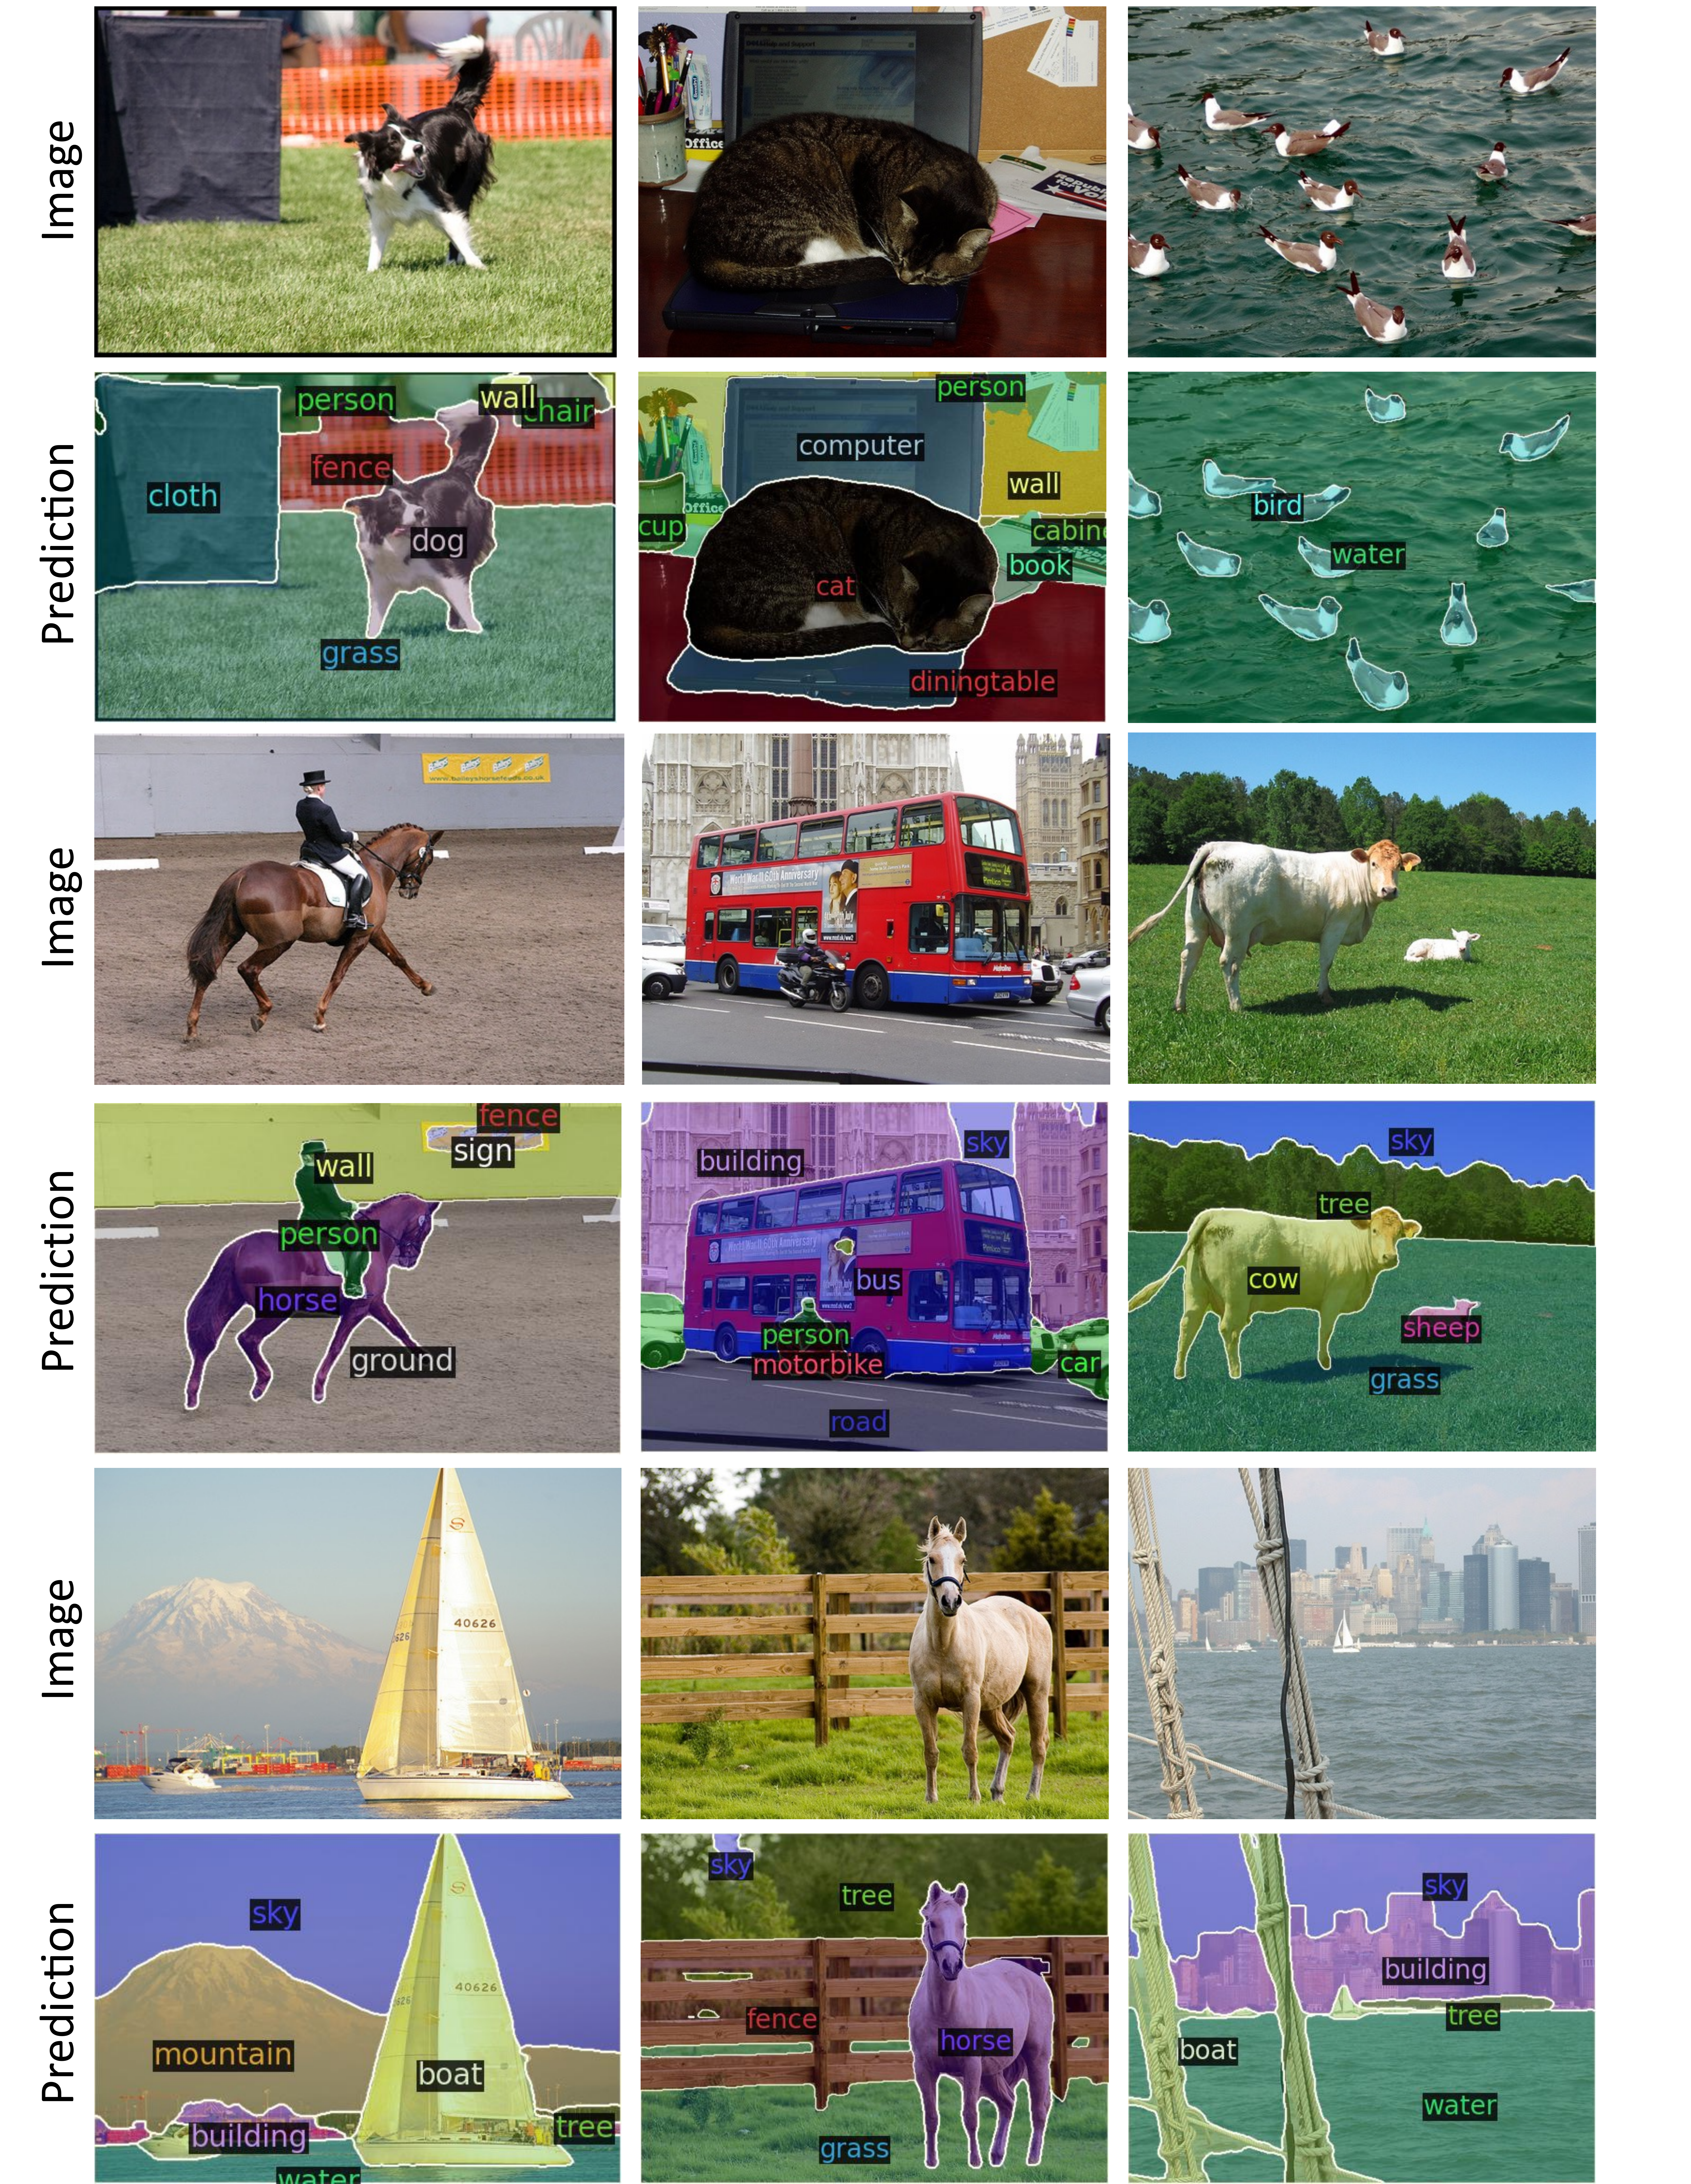}\hfill\\
    \vspace{-5pt}
    \caption{\textbf{Qualitative results on PASCAL Context~\citep{mottaghi2014role} with 59 categories.}}
    \label{fig:pc59}\vspace{-5pt}
\end{figure*}
