# Supplementary material for: CAT-Seg: Cost Aggregation for Open-Vocabulary Semantic Segmentation
Source: arXiv:2303.11797 source file (2024-03-31)
Supplement: Supplementary file 10 [file supp_comparison.tex]

\begin{figure*}
    \centering
    \includegraphics[width=1.0\linewidth]{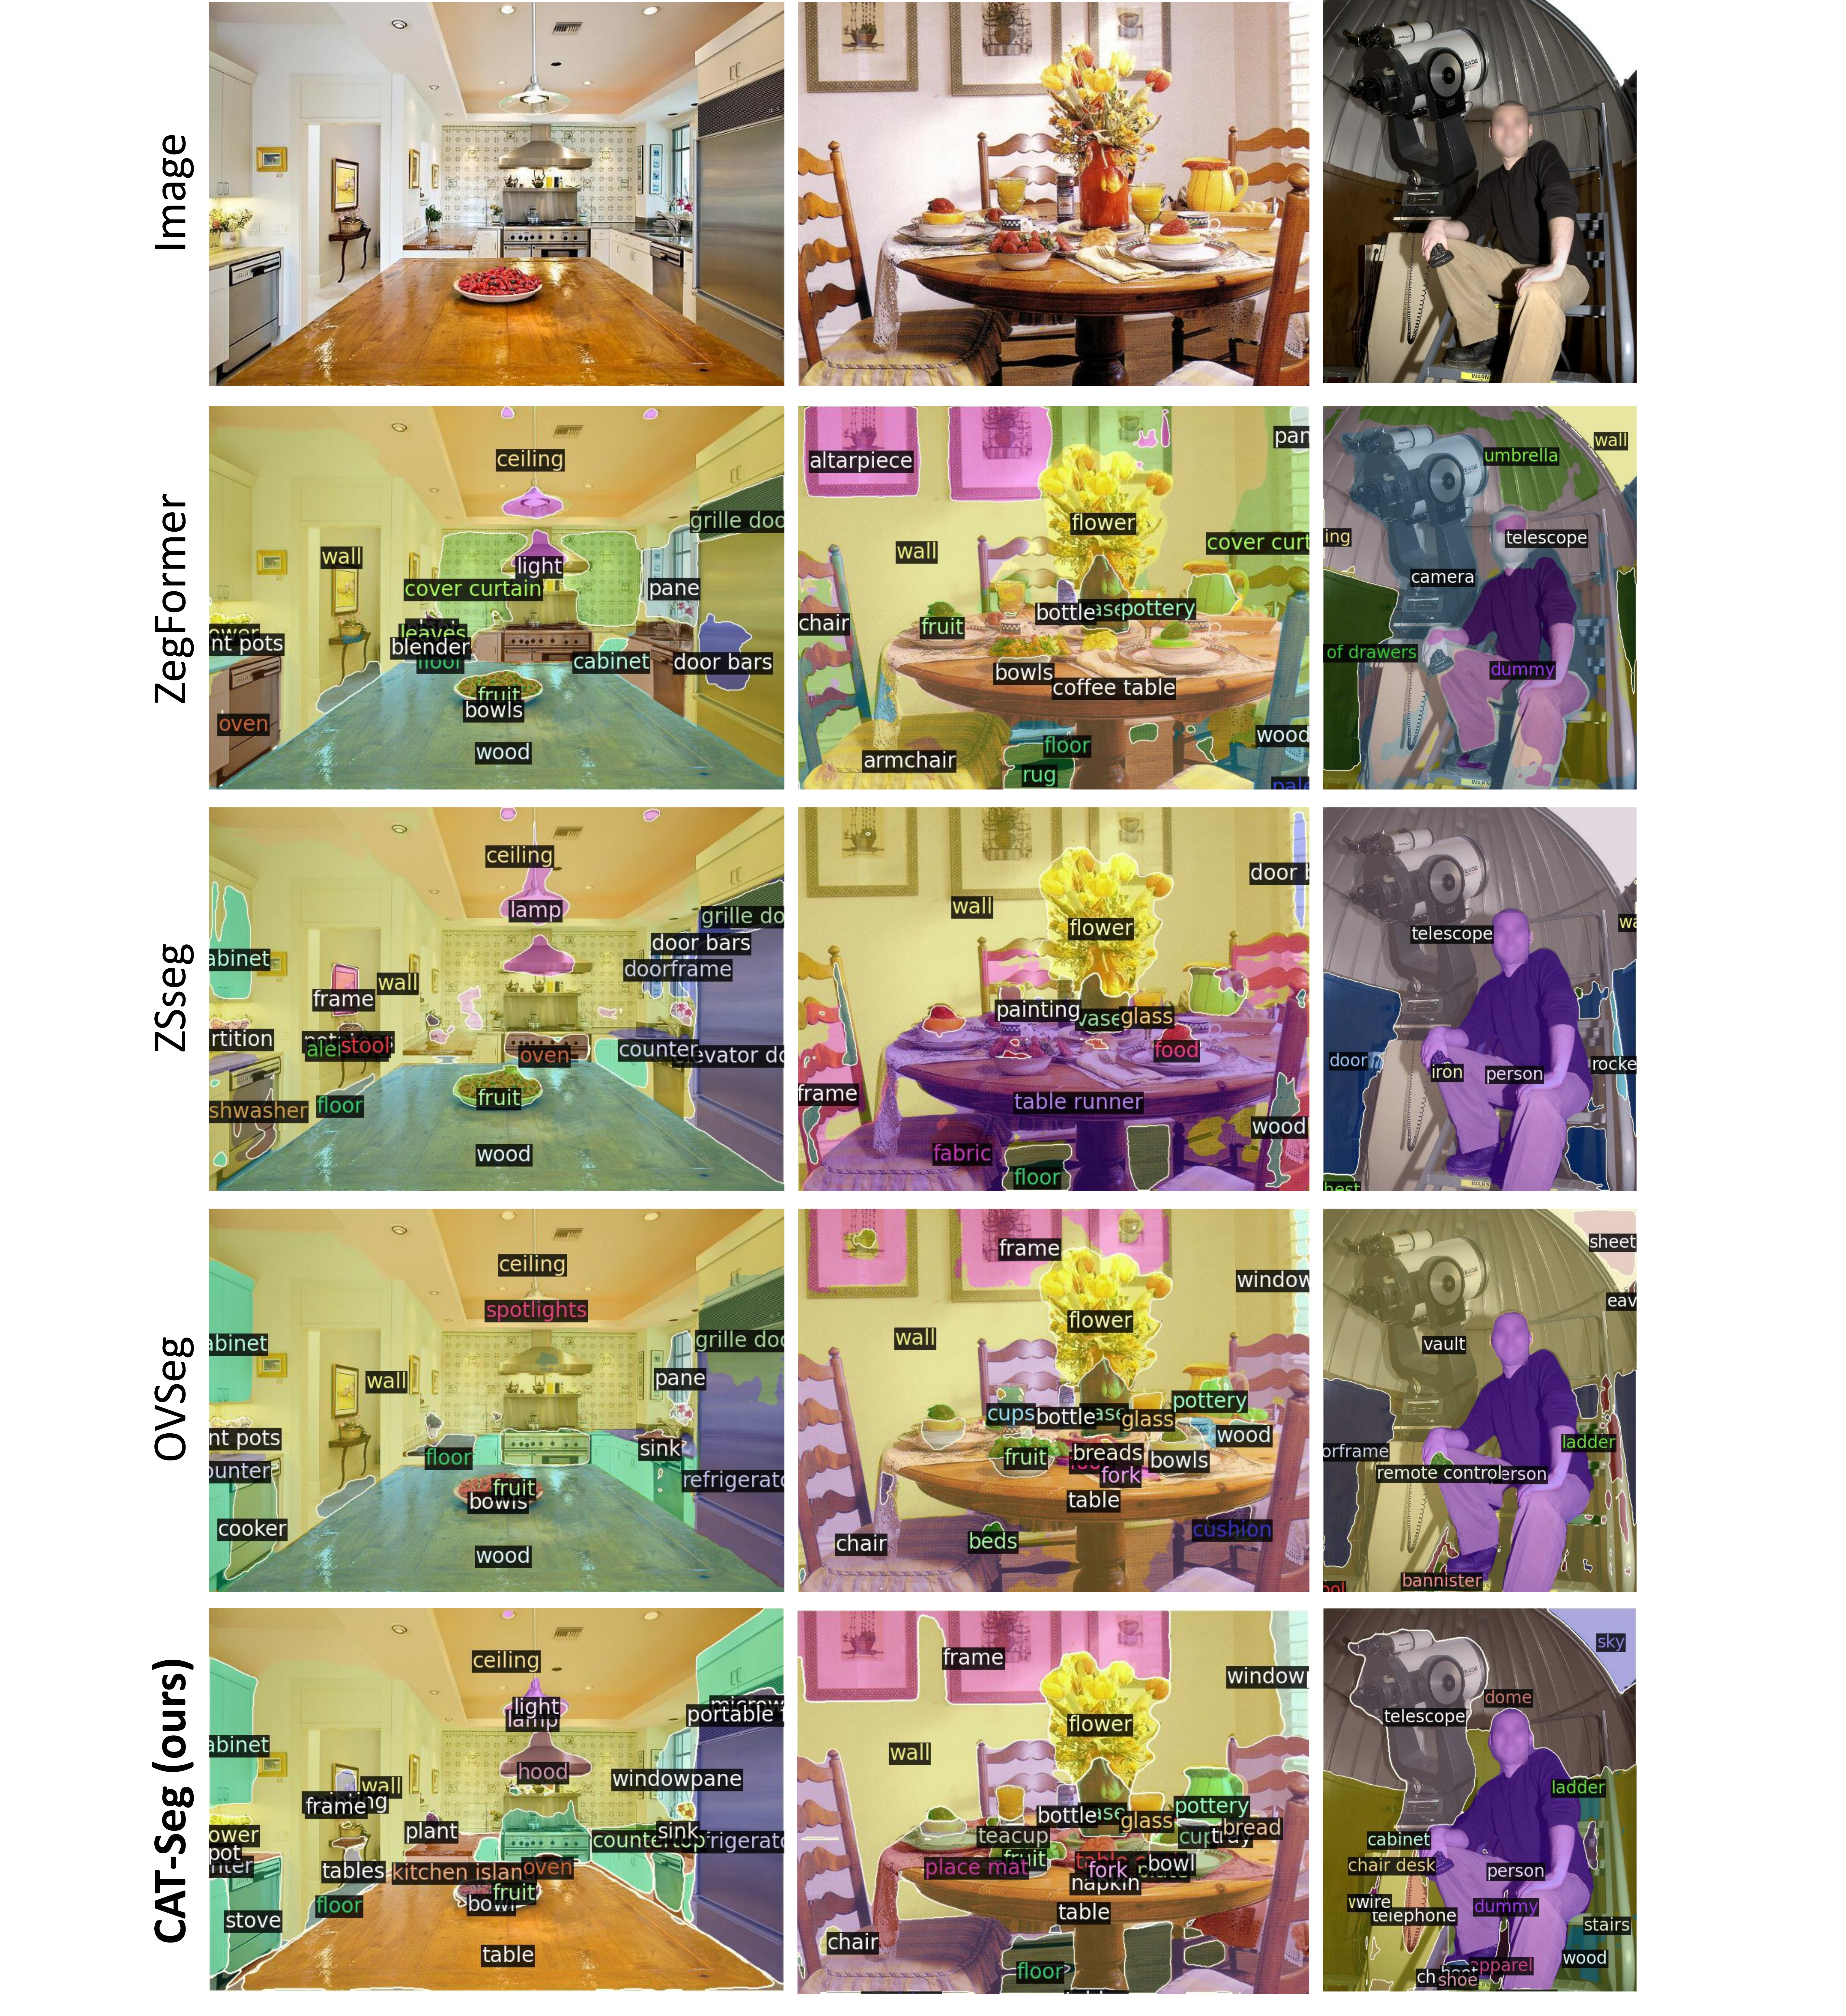}\hfill\\
    \vspace{-5pt}
    \caption{\textbf{Comparison of qualitative results on ADE20K~\citep{zhou2019semantic} with 847 categories.} We compare CAT-Seg with ZegFormer~\citep{ding2022decoupling}, ZSseg~\citep{xu2022simple}, and OVSeg~\citep{liang2022open} on A-847 dataset.}
    \label{fig:ade847-comparison}\vspace{-5pt}
\end{figure*}
