# Supplementary material for: CAT-Seg: Cost Aggregation for Open-Vocabulary Semantic Segmentation
Source: arXiv:2303.11797 source file (2024-03-31)
Supplement: Supplementary file 11 [file vlm.tex]

\begin{table}[H]
\centering
\resizebox{\linewidth}{!}{
\begin{tabular}{l|cccccc}
        \toprule
        VLM & A-847 & PC-459 & A-150 & PC-59 & PAS-20 & $\textnormal{PAS-20}^b$
         \\
        \midrule\midrule
        EVA-02-CLIP-L/14~\cite{sun2023eva} & \underline{16.4} & \underline{24.5} & 37.8 & \underline{62.7} & \textbf{97.9} & \textbf{83.7}\\
        SigLIP-ViT-L/16~\cite{zhai2023sigmoid} & \textbf{18.0}& \textbf{26.1} & \textbf{39.1} & 60.9& \underline{97.2}&80.8\\
        \hlrow CLIP-ViT-L/14 & 16.0 & 23.8 & \underline{37.9} & \textbf{63.3} & 97.0 & \underline{82.5} \\
        \bottomrule
\end{tabular}}
    \vspace{-5pt}
\caption{\textbf{Results on various VLMs.}}
    \vspace{-10pt}
    \label{tab:vlms}
\end{table}
